# Supplementary material for: Patch-based Progressive 3D Point Set Upsampling
Source: arXiv:1811.11286 source file (2019-03-21)
Supplement: Supplementary file 1 [file supplement_content.tex]

%!TEX root = ./ms.tex
This supplementary material provides further technical details and experimental results on an extended dataset (scanned data and ModelNet10). 

\paragraph{Implementation Details.}
By default, we use 16$ \times $-upsampling models with four $ 2\times $ upsampling units.
In each upsampling unit, we implement 4 dense blocks containing 2 dense layers.
The output size of the dense layers $ G $ is set to $ 12 $. 
The compression layer reduces the input prior of each dense block to a fixed number of features $ C' $, and we set $ C'=24 $.
The feature-based KNN inside the dense blocks uses $ K=32 $, while the KNN used during feature interpolation is with $ K=5 $.

The input patches for each upsampling unit have a fixed size $ N $. The choice of $ N $ depends on the size of input shape. For the MNIST contour dataset, $ N = 50 $; for the 3D dataset, $ N = \min(312, \lvert P_0\rvert) $, where $ \lvert P_0\rvert $ is the size of the initial input.

For all experiments, we use a batch size of $ 28 $ and a fixed learning rate of $ 0.001 $. 
Adam optimizer with $ \beta=0.9 $ is used for optimization.

Training 450 epochs using the Sketchfab dataset takes 7 hours on a single GeForce GTX 1080 Ti GPU.
Inference time depends on the number of points in the initial input, the patch size, as well as the number of patches to be extracted in each level.
Typically, performing $ 16\times $ upsampling from 625 and 5000 input points, as shown in Figure~10 and 11 in the main paper, takes about 5 and 18 seconds, respectively.
\begin{figure}[h]
	\centering
	\begin{subfigure}{0.23\linewidth}
		\includegraphics[width=\textwidth]{figures/supplemental/snapshot00}
	\end{subfigure}
	\begin{subfigure}{0.23\linewidth}
		\includegraphics[width=\textwidth]{figures/supplemental/snapshot01}
	\end{subfigure}
	\begin{subfigure}{0.23\linewidth}
		\includegraphics[width=\textwidth]{figures/supplemental/snapshot02}
	\end{subfigure}
	\begin{subfigure}{0.23\linewidth}
		\includegraphics[width=\textwidth]{figures/supplemental/snapshot03}
	\end{subfigure}
	\caption{Examples of generated virtual scans. Such scans are used as training and testing data.}
	\label{fig:scan_inputs}
\end{figure}
\paragraph{Ablation study for the feature extraction unit.}
We conduct experiments to validate the design choice of our feature extraction unit.
The baseline of this study is the PointNet++ \cite{qi2017pointnet++} inspired feature extractor used in PU-Net \cite{yu2018pu} with reduced width, such that the model size is comparable with ours.
We incrementally add one component of our feature extractor and evaluate the chamfer distance and hausdorff distance.
As shown in Table~\ref{tab:feature_extraction}, all components consistently improvement the upsampling quality in both metrics.
When combined together, our feature extractor significantly outperforms the baseline model with fewer parameters.

\begin{table}[h]\small\centering
	\begin{tabular}{lllll}
		\toprule
		& feature extraction unit & CD $ \cdot 10^{-3} $ & HD $ \cdot 10^{-3} $& \# Params \\\midrule
		1)& narrow PU-Net & 0.93 & 11.47 & 513K \\
		2)& 1) + feature-based $ k $NN & 0.86 & 9.83 & 554K \\
		3)& 2) + w/o subsample & 0.62 & 7.89 & 387K \\
		%4)& 3) + intra-block dense link & 0.76 & 8.64 & 255K \\
		4)& 3) + dense links & 0.54 & 6.92 & 304K \\
		\bottomrule
	\end{tabular}\vspace{-8pt}
	\caption{Ablation study for the feature extraction unit. The baseline is the PointNet++ based feature extractor used in PU-Net; we reduced the width of this network for comparable network capacity.}\label{tab:feature_extraction}
\end{table}
\paragraph{Upsampling of scanned data.}
We extend our model to handle scanned data by synthesizing a large amount of training data similar to real scans.
We implement a virtual scanner to scan the training set of the Sketchfab dataset from a random viewpoint using different camera resolutions.
By gradually increasing the camera resolution, we obtain a list of virtual scans with increasing density, as shown in Figure~\ref{fig:scan_inputs}.

We test the trained model on both virtual and real scans. The results are shown in Figure~\ref{fig:scan_results} and \ref{fig:real_results}.
The virtual scans are generated from the testing set of the Sketchfab dataset, while the real scans are acquired via the Intel RealSense SR300 scanner. As an alternative to the WLOP consolidation, we use the scanner's built-in filter to obtain a relatively clean input, which typically smears the fine-grained details and reduces the frame rate. 
As shown in Figure~\ref{fig:scan_results}, our model is able to reveal fine-grained geometry from very sparse inputs.
In addition, it can fill holes and preserve sharp features, as shown in Figure~\ref{fig:real_results}.
\begin{figure}[h]
	\centering
	\includegraphics[width=0.95\linewidth]{figures/supplemental/scan}
	\caption{$ 16\times $ upsampling results on virtual scans.}\label{fig:scan_results}
\end{figure}
\begin{figure}[h]
	\centering
	\includegraphics[width=0.95\linewidth]{figures/supplemental/real_scan}
	\caption{$ 16\times $ upsampling results on real scans.}\label{fig:real_results}
\end{figure}

%\section{Extended experiments.}
%\paragraph{Generalization.}
%Since all levels of details are upsampled patch-wise in our network, the upsampling result is robust with respect to the global shape.
%We demonstrate this point quantitatively using ModelNet10 \cite{wu20153d}.
%Specifically, we train a $ 8\times $ network using the training examples from ``chair" category and test the trained model on all categories.
%Same as Sketchfab dataset, the input and reference points are sampled from CAD meshes using Poisson-disk sampling.
%
%As Table~\ref{tab:modelnet} shows, the performance of our model is unbiased for any particular category, suggesting that it is robust under global shape variation.
%\begin{table}
%	\footnotesize
%	\setlength{\tabcolsep}{2pt}
%	\def\arraystretch{1.5}
%	\begin{tabular}{l*{10}{c}}
%		\toprule
%		& bathtub & bed & chair & desk & dresser & monitor & \makecell{night\\stand} & sofa & table & toilet \\\midrule
%		\makecell{CD \\$ 10^{-4} $} & 8.22 & 9.41 & 8.65 & 9.63 & 12.05 & 8.06 & 13.64 & 9.26 & 5.64 & 11.00
%		\\\bottomrule
%	\end{tabular}
%	\caption{Generalizability test on ModelNet10 using chamfer loss. We train a $ 8\times $ upsampling model using ``chair" category from ModelNet10 and test it on the test data of all 10 categories. }
%	\label{tab:modelnet}
%\end{table}

\paragraph{Upsampling on ModelNet10.}
In addition to the quantitative evaluation on ModelNet10 shown in the main paper, we provide some examples for qualitative comparision.
As shown in Figure~\ref{fig:modelnet}, we randomly pick one model from each category as input. 
The output points are color-coded based on the nearest neighbor distance to the ground truth.
Similar to what is demonstrated in Table~1 of the main paper, EC-Net has difficulty handling sparse inputs.
Overall, our model significantly outperforms PU-Net and EC-Net in this experiment.

\begin{figure*}
	\centering
\setlength{\tabcolsep}{2pt}
\let\mytmplen\relax
\newlength{\mytmplen}
\setlength\mytmplen{0.09\textheight}
\begin{tabular}{cccc}
\includegraphics[height=\mytmplen]{figures/supplemental/modelnet/bathtub_input1}&
\includegraphics[height=\mytmplen]{figures/supplemental/modelnet/bathtub_pu1}&
\includegraphics[height=\mytmplen]{figures/supplemental/modelnet/bathtub_ec1}&
\includegraphics[height=\mytmplen]{figures/supplemental/modelnet/bathtub_ours1}\\
\includegraphics[height=\mytmplen]{figures/supplemental/modelnet/bed_input01}&
\includegraphics[height=\mytmplen]{figures/supplemental/modelnet/bed_pu01}&
\includegraphics[height=\mytmplen]{figures/supplemental/modelnet/bed_ec01}&
\includegraphics[height=\mytmplen]{figures/supplemental/modelnet/bed_ours01}\\
\includegraphics[height=\mytmplen]{figures/supplemental/modelnet/chair_input00}&
\includegraphics[height=\mytmplen]{figures/supplemental/modelnet/chair_pu00}&
\includegraphics[height=\mytmplen]{figures/supplemental/modelnet/chair_ec00}&
\includegraphics[height=\mytmplen]{figures/supplemental/modelnet/chair_ours00}\\
\includegraphics[height=\mytmplen]{figures/supplemental/modelnet/desk_input00}&
\includegraphics[height=\mytmplen]{figures/supplemental/modelnet/desk_pu00}&
\includegraphics[height=\mytmplen]{figures/supplemental/modelnet/desk_ec00}&
\includegraphics[height=\mytmplen]{figures/supplemental/modelnet/desk_ours00}\\
\includegraphics[height=\mytmplen]{figures/supplemental/modelnet/dresser_input00}&
\includegraphics[height=\mytmplen]{figures/supplemental/modelnet/dresser_pu00}&
\includegraphics[height=\mytmplen]{figures/supplemental/modelnet/dresser_ec00}&
\includegraphics[height=\mytmplen]{figures/supplemental/modelnet/dresser_ours00}\\
\includegraphics[height=\mytmplen]{figures/supplemental/modelnet/monitor_input00}&
\includegraphics[height=\mytmplen]{figures/supplemental/modelnet/monitor_pu00}&
\includegraphics[height=\mytmplen]{figures/supplemental/modelnet/monitor_ec00}&
\includegraphics[height=\mytmplen]{figures/supplemental/modelnet/monitor_ours00}\\
\includegraphics[height=\mytmplen]{figures/supplemental/modelnet/nightstand_input00}&
\includegraphics[height=\mytmplen]{figures/supplemental/modelnet/nightstand_pu00}&
\includegraphics[height=\mytmplen]{figures/supplemental/modelnet/nightstand_ec00}&
\includegraphics[height=\mytmplen]{figures/supplemental/modelnet/nightstand_ours00}\\
\includegraphics[height=\mytmplen]{figures/supplemental/modelnet/sofa_input00}&
\includegraphics[height=\mytmplen]{figures/supplemental/modelnet/sofa_pu00}&
\includegraphics[height=\mytmplen]{figures/supplemental/modelnet/sofa_ec00}&
\includegraphics[height=\mytmplen]{figures/supplemental/modelnet/sofa_ours00}\\
\includegraphics[height=\mytmplen]{figures/supplemental/modelnet/table_input00}&
\includegraphics[height=\mytmplen]{figures/supplemental/modelnet/table_pu00}&
\includegraphics[height=\mytmplen]{figures/supplemental/modelnet/table_ec00}&
\includegraphics[height=\mytmplen]{figures/supplemental/modelnet/table_ours00}\\
\includegraphics[height=\mytmplen]{figures/supplemental/modelnet/toilet_input00}&
\includegraphics[height=\mytmplen]{figures/supplemental/modelnet/toilet_pu00}&
\includegraphics[height=\mytmplen]{figures/supplemental/modelnet/toilet_ec00}&
\includegraphics[height=\mytmplen]{figures/supplemental/modelnet/toilet_ours00}\\
input & PU-Net & EC-Net & Ours
\end{tabular}
\caption{Upsampled examples of ModelNet10. The color encodes the distance to the closest neighbor in ground truth.}\label{fig:modelnet}
\end{figure*}
